# Supplementary material for: MixDiT: Accelerating Image Diffusion Transformer Inference with Mixed-Precision MX Quantization
Source: arXiv:2504.08398 source file (2025-04-11)
Supplement: Supplementary file 1 [file appendix.tex]

{\appendix[Proof of the XYZ Equation]}
